# Supplementary material for: StructChart: On the Schema, Metric, and Augmentation for Visual Chart Understanding
Source: arXiv:2309.11268 source file (2024-12-04)
Supplement: Supplementary file 1 [file supp.tex]

\newpage
\clearpage

{\appendix

\section*{LLM-based Self-inspection Data Production Scheme}
\label{app:simulation}
The complete schematic simulation process can be divided into two stages, containing (1) Data simulation stage for label generation. (2) Image simulation stage for chart generation. We demonstrate the completed prompts in Table~\ref{fig:simulation_2}.

\section*{In-depth analysis of Real \& Sim chart data}
1) We compared our Simchart9K with real data proposed in this work (ChartQA, PlotQA, Chart2Text):
\begin{itemize}
    \item All the datasets cover three regular chart types, including line chart, bar chart, and pie chart.
    \item Fig.~\ref{fig:tsne} reveals that although there are obvious pixel-level feature distribution differences between real data sets, SimChart9K can better cover the distribution of all data sets.
    \item All images in SimChart9K are drawn by Python code, but some images in the real data set also use other visualization tools.
\end{itemize}

2) We compared our Simchart9K with other in-the-wild real data:
\begin{itemize}
    \item There are more chart types in the real world such as radar charts, heatmaps, funnel charts, 3D bar charts, etc.
    \item  Real-world chart styles are more diverse. In addition to using code and visualization tools, there will also be more conceptual designs.
    \item There will be more high-order information (i.e. relationship between multiple entities) in the real-world charts (i.e. 3D charts or multi-charts)
\end{itemize}

%-------------------------------------------------------------------------------------------------------------

% \section*{Visualization Comparisons with Matcha and Deplot}
% \label{app:compare_matcha}
% We compare the proposed Structchart with Matcha~\citep{Liu2022MatChaEV} and Deplot~\citep{Liu2022DePlotOV} in Chart Information Extraction (CIE) task in Figs.~\ref{fig:vis_compare_1},~\ref{fig:vis_compare_2} and~\ref{fig:vis_compare_3}. Matcha~\citep{Liu2022MatChaEV} cannot perform the CIE task and can only output the content in the form of HTML format during the pre-training phase, and Deplot~\citep{Liu2022DePlotOV} is affected by noisy backgrounds (\textit{e.g.} web page environment containing other irrelevant text). By comparison, our Structchart can extract accurate information of the chart from complicated backgrounds, such as information from the website.

\section*{More Results of StructChart on Different Downstream Tasks}
\label{app:different_task}
We visually demonstrate StructChart on downstream tasks in Figs.~\ref{fig:multi_task_1},  including Question Answering (QA), summarization, and redrawing. For the QA task, quantitative evaluation results are shown in Tab~\ref{tab:qa}, and here, we further give many visualization results. For the summarization task, some open-ended summary descriptions can be conducted beyond the basic numeric description. For redrawing, different types of charts can be obtained by redrawing chart images given the statistical data (\textit{e.g.}, line chart $\to$ bar chart, bar chart $\to$ pie chart, \textit{etc.}). We also provide visualization performance of StructChart on some in-the-wild chart images in Fig.~\ref{fig:ood}.

\section*{Demonstrations on Downstream tasks with Linear CSV Tokens (LCT) v.s. Structured Triplet Representations (STR) }
\label{app:compare_lct_str}
We respectively use Linear CSV Tokens (LCT) and Structured Triplet Representations (STR) as intermediate representations of chart information for different downstream tasks. Figs.~\ref{fig:lct_str_1} and \ref{fig:lct_str_2} show that STR used in StructChart has better robustness compared to LCT. When noise is introduced into the highly position-sensitive LCT (a comma is introduced as noise as illustrated in Fig.~\ref{fig:lct_str_1}, and the separator comma itself is included as illustrated in Fig.~\ref{fig:lct_str_2}), all downstream tasks will be affected negatively. By comparison, our StructChart achieves better performance on QA, summarization, and redrawing tasks, owing to the proposed STR.

\section*{Comparisons with Other General Vision Language Models (VLM) on Downstream Tasks}
\label{app:gpt4v}
We demonstrate three visualization comparisons among StrcutChart, GPT-4V~\citep{OpenAI2023GPT4TR} and LLaVA-1.5~\citep{Liu2023VisualIT} for downstream tasks in Figs.~\ref{fig:gpt4v_1} and~\ref{fig:gpt4v_2}. It is worth noting that for the QA task, our StructChart is restricted to generating answers only in order to report the quantitative results on the ChartQA dataset. From the visualization results, it can be seen that the proposed StructChart has a strong Chart-based reasoning ability, showing promising performance on multiple downstream tasks. Although GPT-4V~\citep{OpenAI2023GPT4TR} also has a strong performance, our model weights, training code, simulation code, and simulation dataset will all be open-sourced.

\section*{Discussion About How To Obtain General Chart Large Model (CLM)}
Here, we discuss one possible direction for training a Chart Large Model (CLM), which is challenging due to: (1) Scarce chart data covering as comprehensive scientific fields as possible, and (2) the Perception-reasoning task gap. This paper provides a preliminary attempt to tackle the above challenges. In the future, we intend to collect more chart data from different scientific subjects and perform the proposed LLM-based self-inspection data production scheme to enhance chart data diversity. This would be the foundation for training a general CLM with a large amount of simulated chart data which are rendered using real-world chart data from multiple fields.

\begin{table*}[t]
    \centering
    \small
     % Adjust column space
    \caption{Prompts of label-efficient chart simulation process including (1) data simulation stage for labels generation. (2) image simulation stage for chart generation.}
    \label{fig:simulation_2}
    % \resizebox{0.9\textwidth}{!}{  % Resize the table to fit within the text width
    \begin{tabular}{c|p{12cm}}  % Use 12cm or adjust column width accordingly
     \toprule
     \textbf{Stage} & \textbf{Prompt}\\
     \midrule
    \textit{Data Simulation}  & 
     \begin{minipage}[t]{\textwidth}  % Auto-adjust minipage width
     \textbf{System Prompt:} Copying the following table information can be expanded and adapted as\\
     appropriate, The imitation is as irrelevant as possible to the original text.\\
     
    \textbf{Input Data}: The data is \texttt{<data> \{data\_LCT\} </data>}
     \end{minipage}
     \\
     \midrule
    \textit{Image Simulation}  & 
     \begin{minipage}[t]{\textwidth}  % Auto-adjust minipage width
     \textbf{System Prompt:}      
            Consider you are a professional Python grapher.\\
            Please draw and save a chart based on the following data using Python, and images must be \\
            clear and intuitive.\\  
            Choose a plot type that best suits the value, for example, line, column, scatter, and pie charts.\\ 
            Drawing techniques such as background grids can be used.\\
            Draw as much variety as possible.\\
            Clear the current image state at the end of the code.\\
            If the text length of the label is too long, use the method of adding the parameter \texttt{rotation}\\
            or display label on separate lines seting \texttt{wrap=true}.\\
            The figsize parameter is set to a larger setting to prevent content from being displayed. \\
            Automatically resize the image by \texttt{tight\_layout()}.\\
            You must use xticks to prevent interpolation.\\
            Do not set special fonts such as sans-serif and Arial etc. to avoid the problem of missing fonts.\\
            If the string in the picture is too long, find a way for all characters to show and not be\\
            overwritten and stacked on top of each other.\\
            Do not have extra leading words at the beginning and end of the generated code, such as\\
            \texttt{python code, python, ```}, etc.\\
            Check the generated code without errors, do not include undefined functions.\\

    \textbf{Data:}The data is \texttt{<data> \{data generated in previous stage\} </data>}
    \end{minipage}
    \\
    \bottomrule
    \end{tabular}
    % }  % End of resizebox
\end{table*}

%___________________________________________________________________________________%

%-----------------------------------

% \begin{figure*}[tb!]
% \centering
% \includegraphics[width=0.92\linewidth]{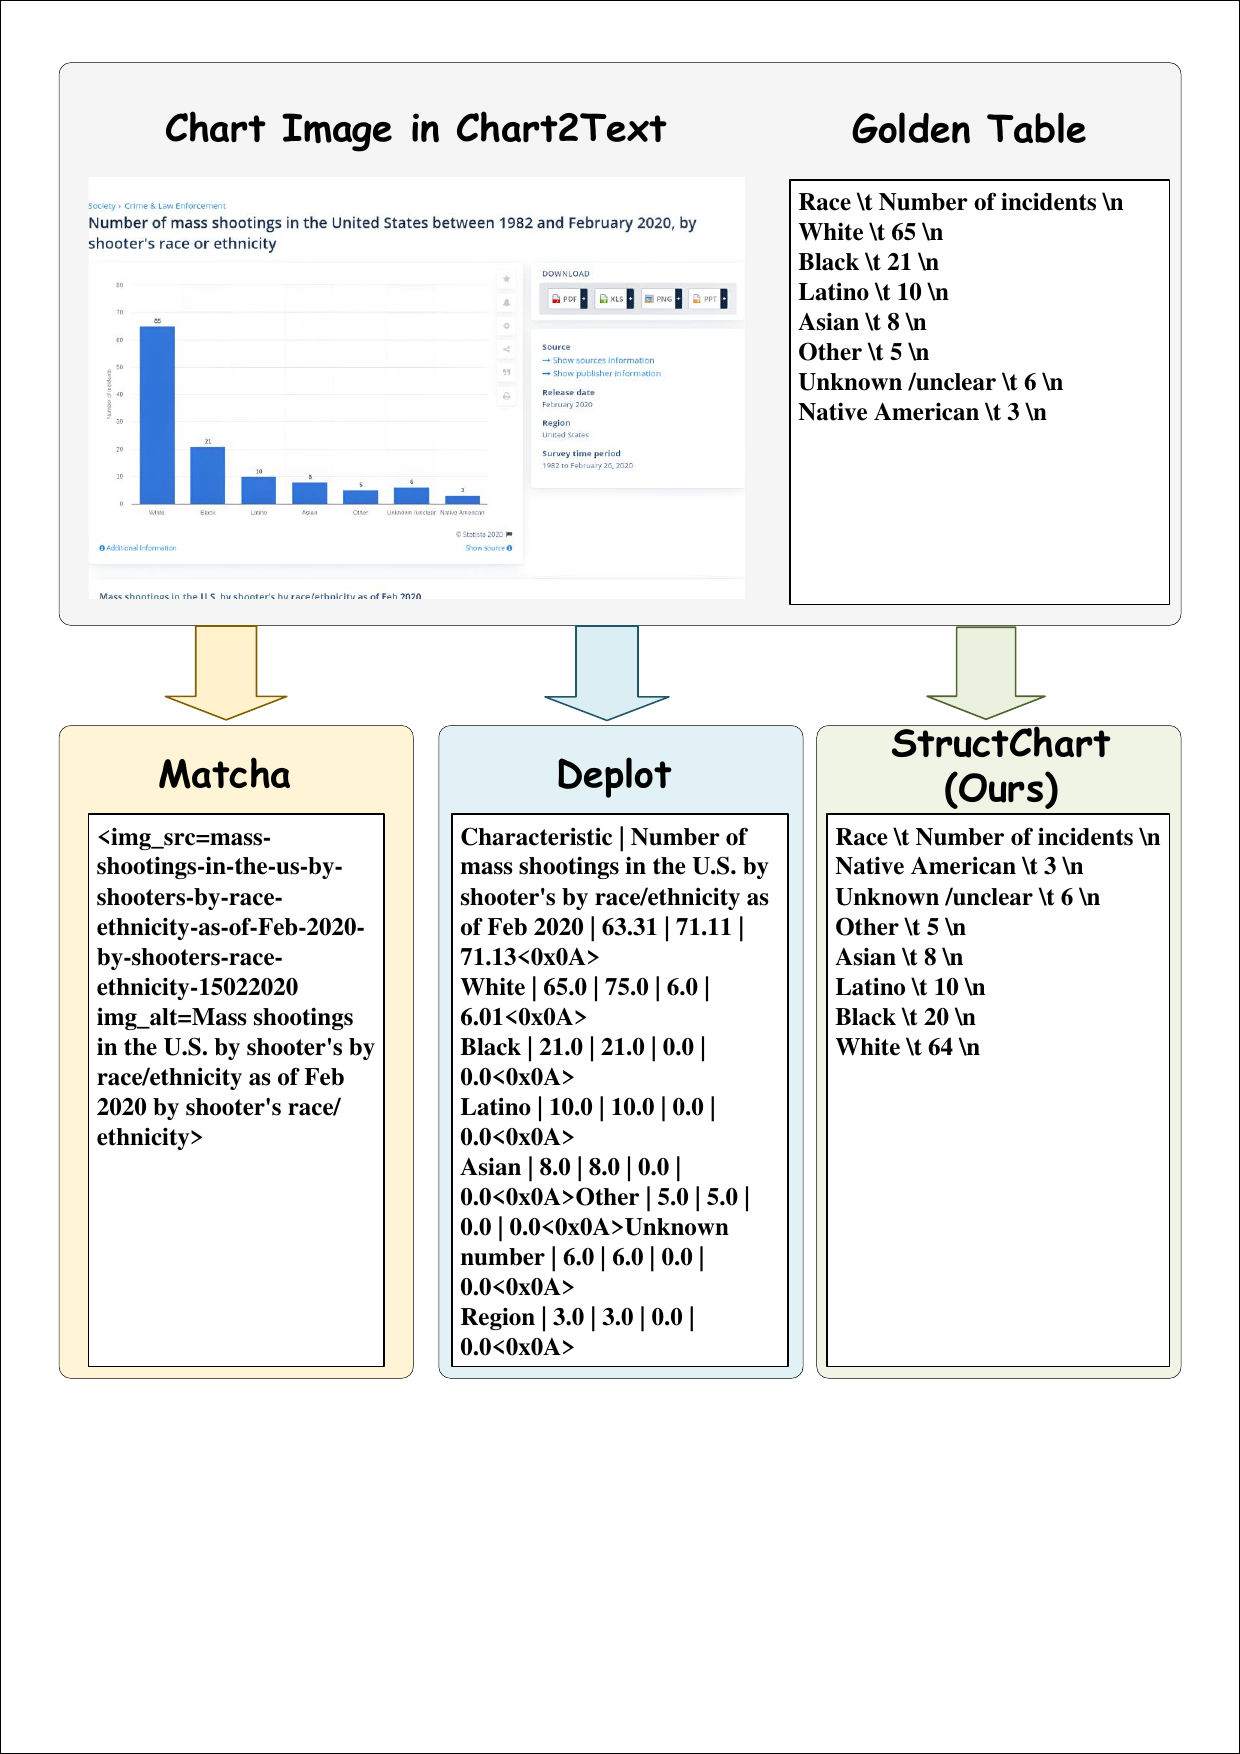}
% \vspace{-5pt}
% \caption{Comparison of the proposed StructChart, Matcha~\citep{Liu2022MatChaEV} and Deplot~\citep{Liu2022DePlotOV}, where the Golden Table represents the ground truth of the parsed chart information.}
% \label{fig:vis_compare_1}
% \end{figure*}

% \begin{figure*}[tb!]
% \centering
% \includegraphics[width=0.92\linewidth]{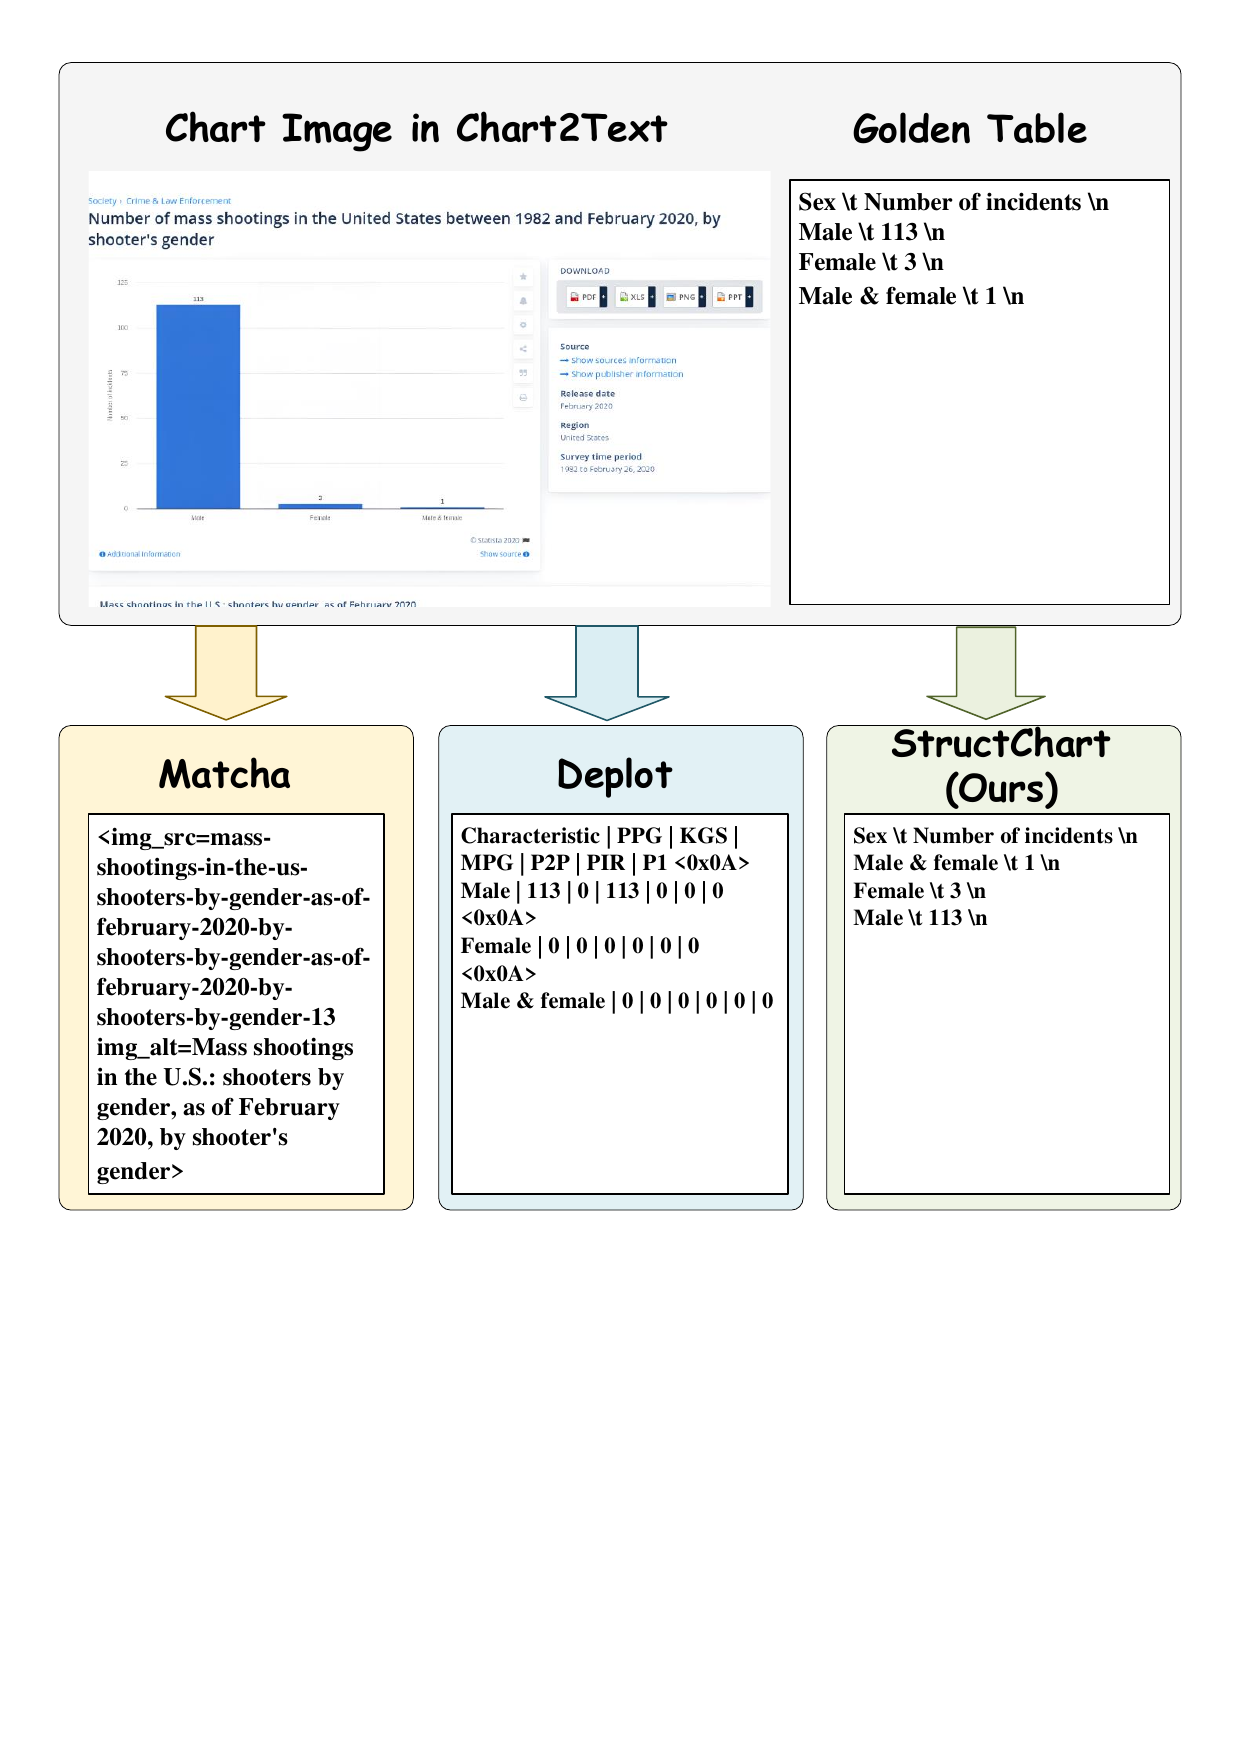}
% \vspace{-5pt}
% \caption{Comparison of the proposed StructChart, Matcha~\citep{Liu2022MatChaEV} and Deplot~\citep{Liu2022DePlotOV}, where the Golden Table represents the ground truth of the parsed chart information.}
% \label{fig:vis_compare_2}
% \end{figure*}

% \begin{figure*}[tb!]
% \centering
% \includegraphics[width=0.92\linewidth]{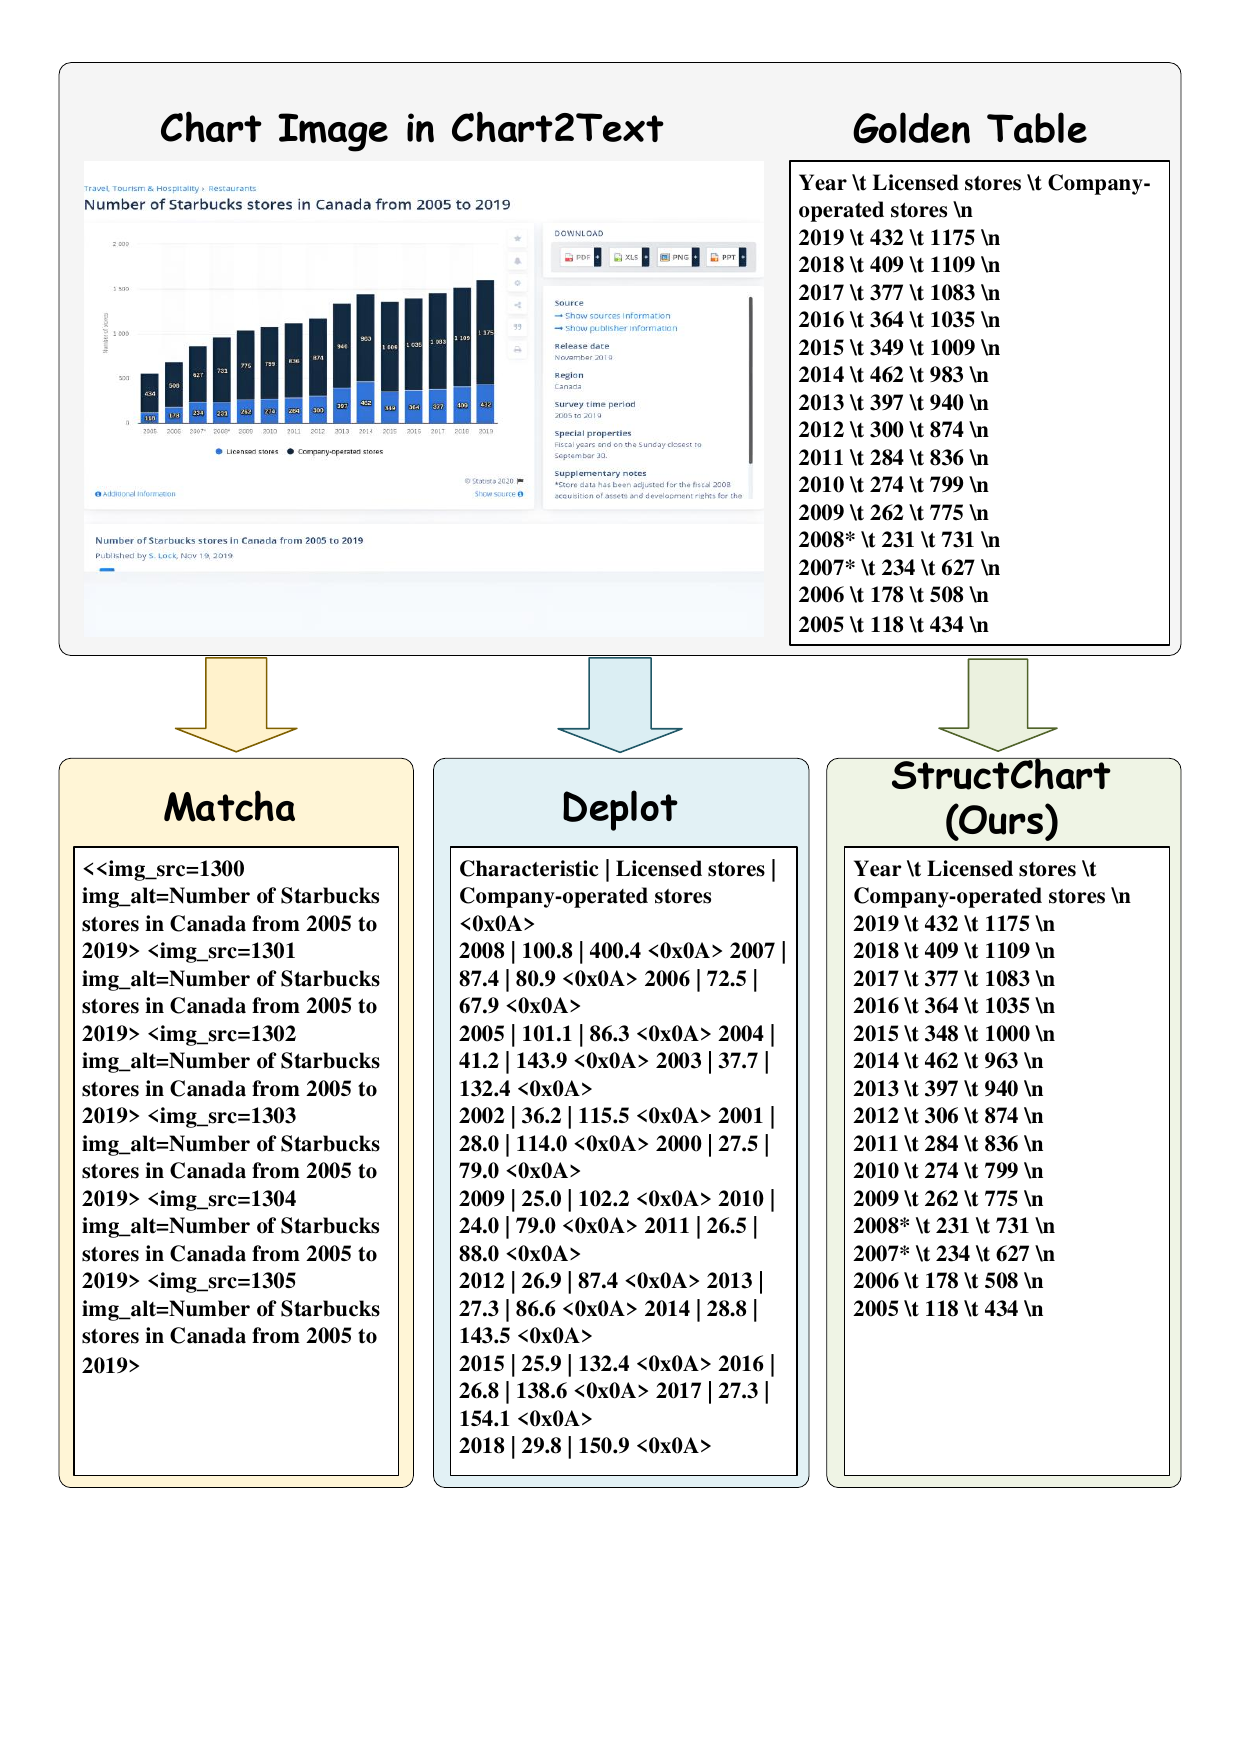}
% \vspace{-5pt}
% \caption{Comparison of the proposed StructChart, Matcha~\citep{Liu2022MatChaEV} and Deplot~\citep{Liu2022DePlotOV}, where the Golden Table represents the ground truth of the parsed chart information.}
% \label{fig:vis_compare_3}
% \end{figure*}

\begin{figure}[tb!]
\centering
\includegraphics[width=0.88\linewidth]{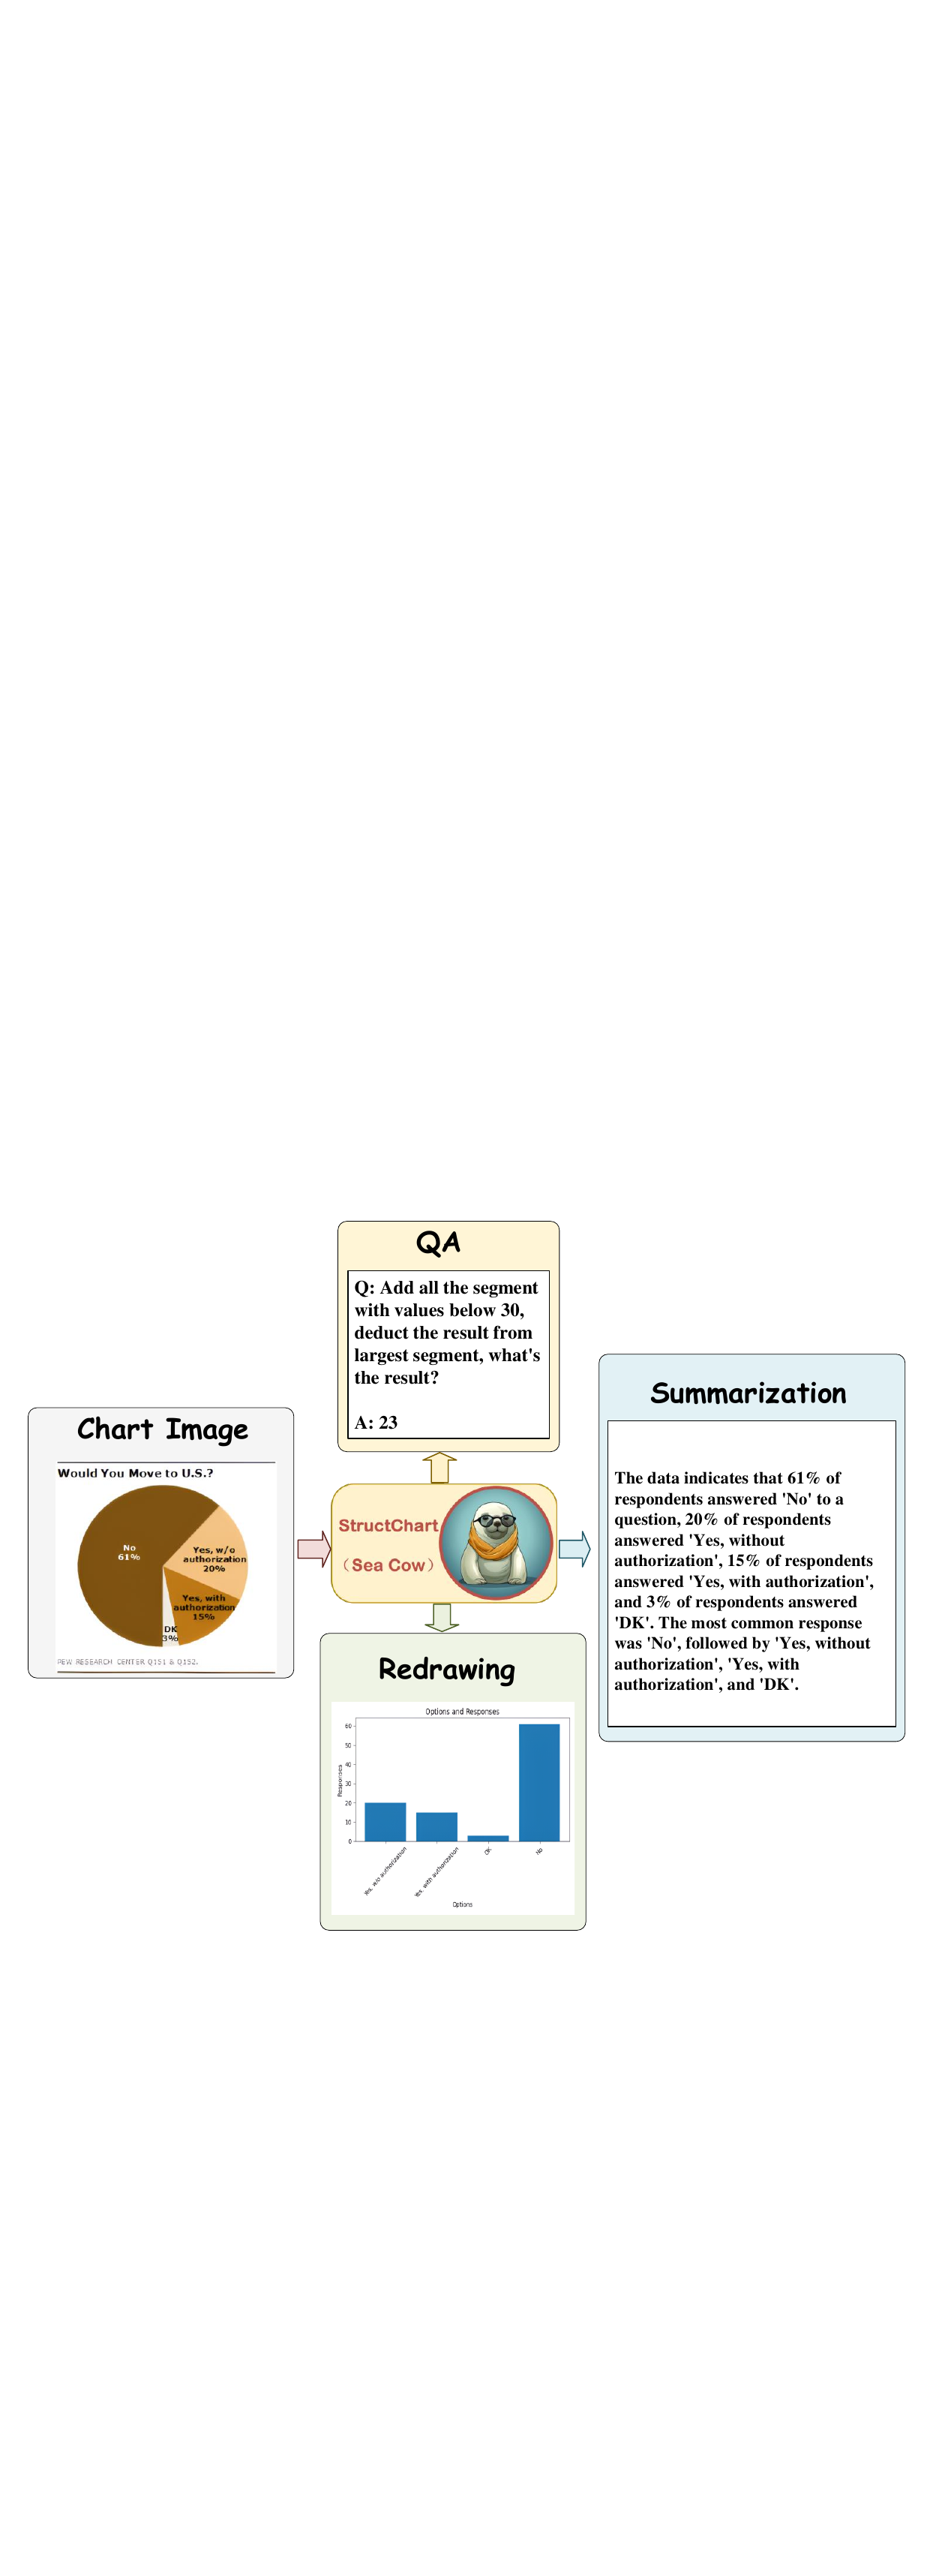}
\vspace{-5pt}
\caption{Visualization results using the proposed StructChart on different chart-related reasoning tasks including Question Answering (QA), Summarization, and Redrawing.}
\label{fig:multi_task_1}
\end{figure}

% \begin{figure}[tb!]
% \centering
% \includegraphics[width=0.8\linewidth]{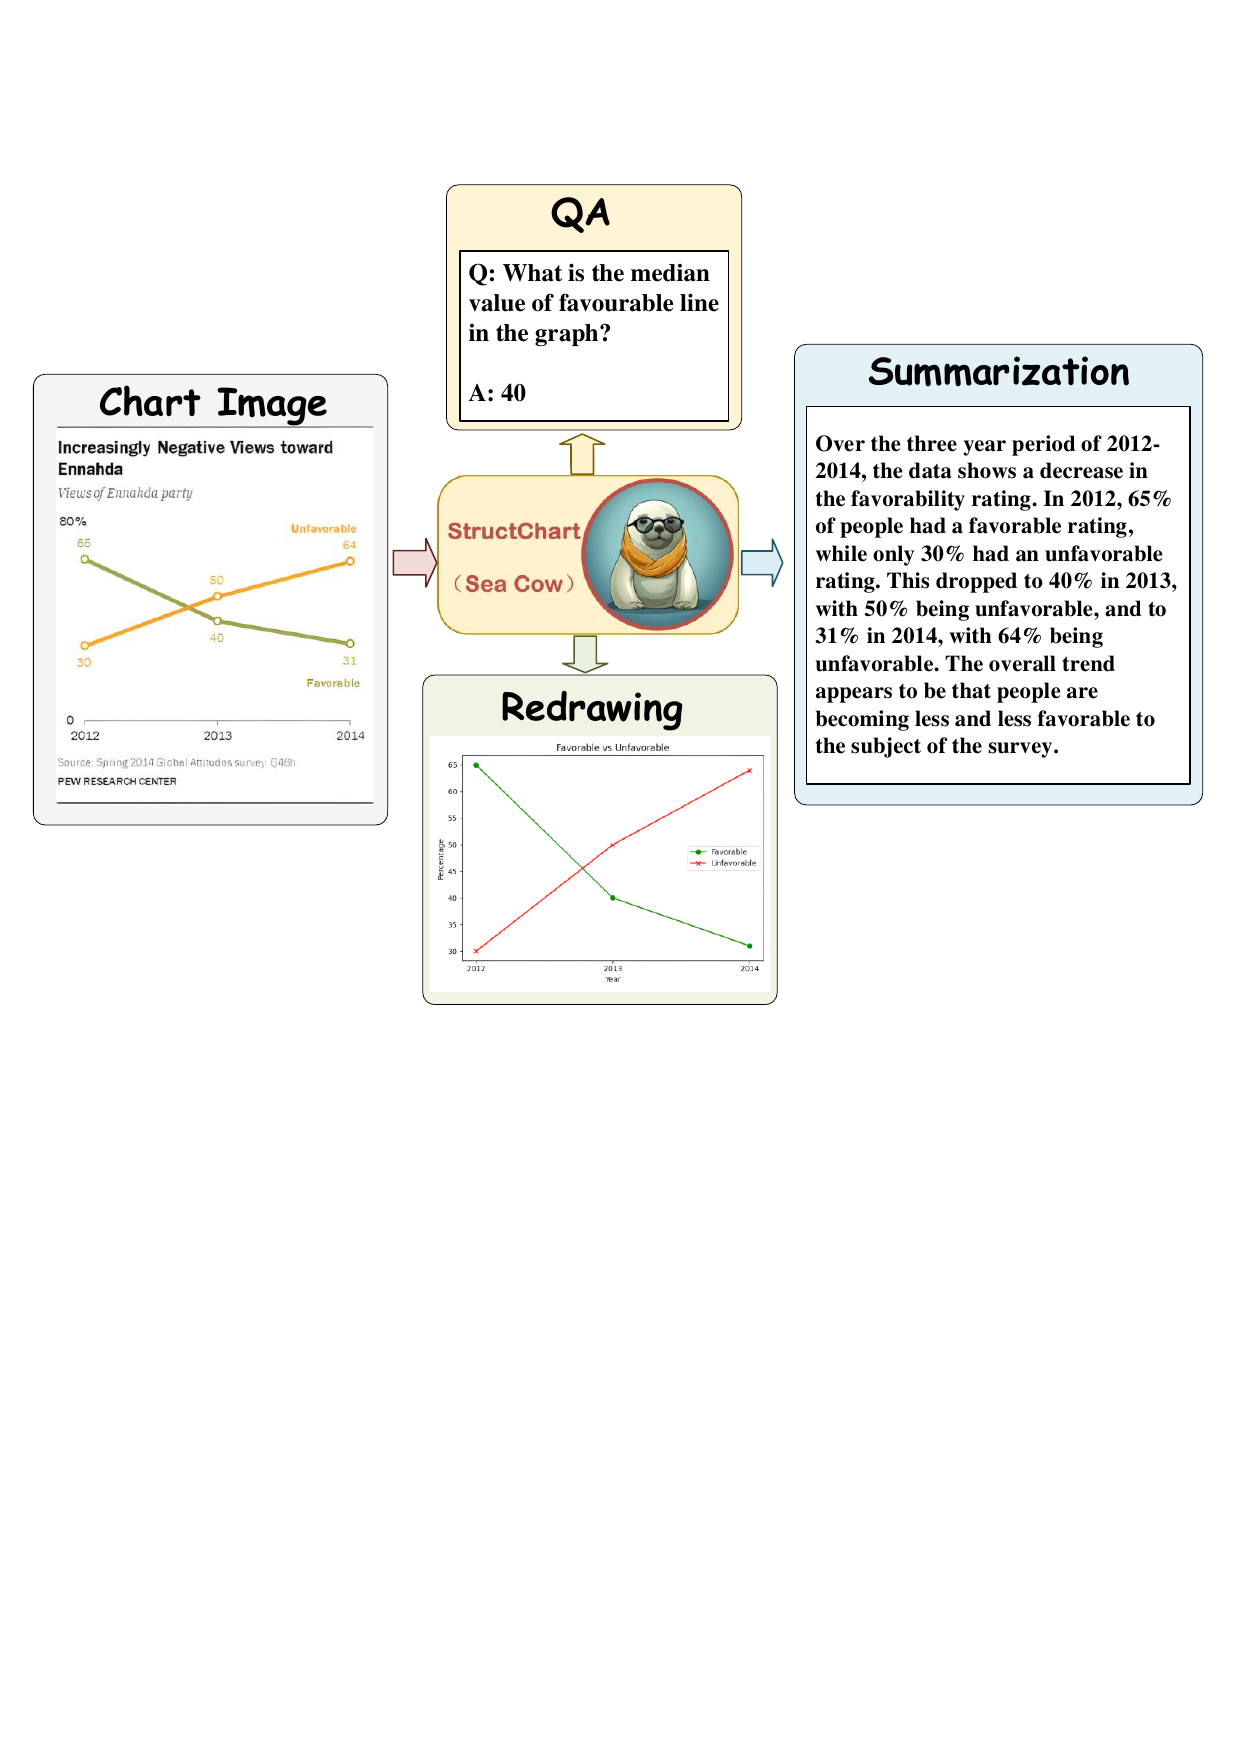}
% \vspace{-5pt}
% \caption{Visualization results using the proposed StructChart on different chart-related reasoning tasks including Question Answering (QA), Summarization, and Redrawing.}
% \label{fig:multi_task_2}
% \end{figure}

\begin{figure}[tb!]
\centering
\includegraphics[width=0.88\linewidth]{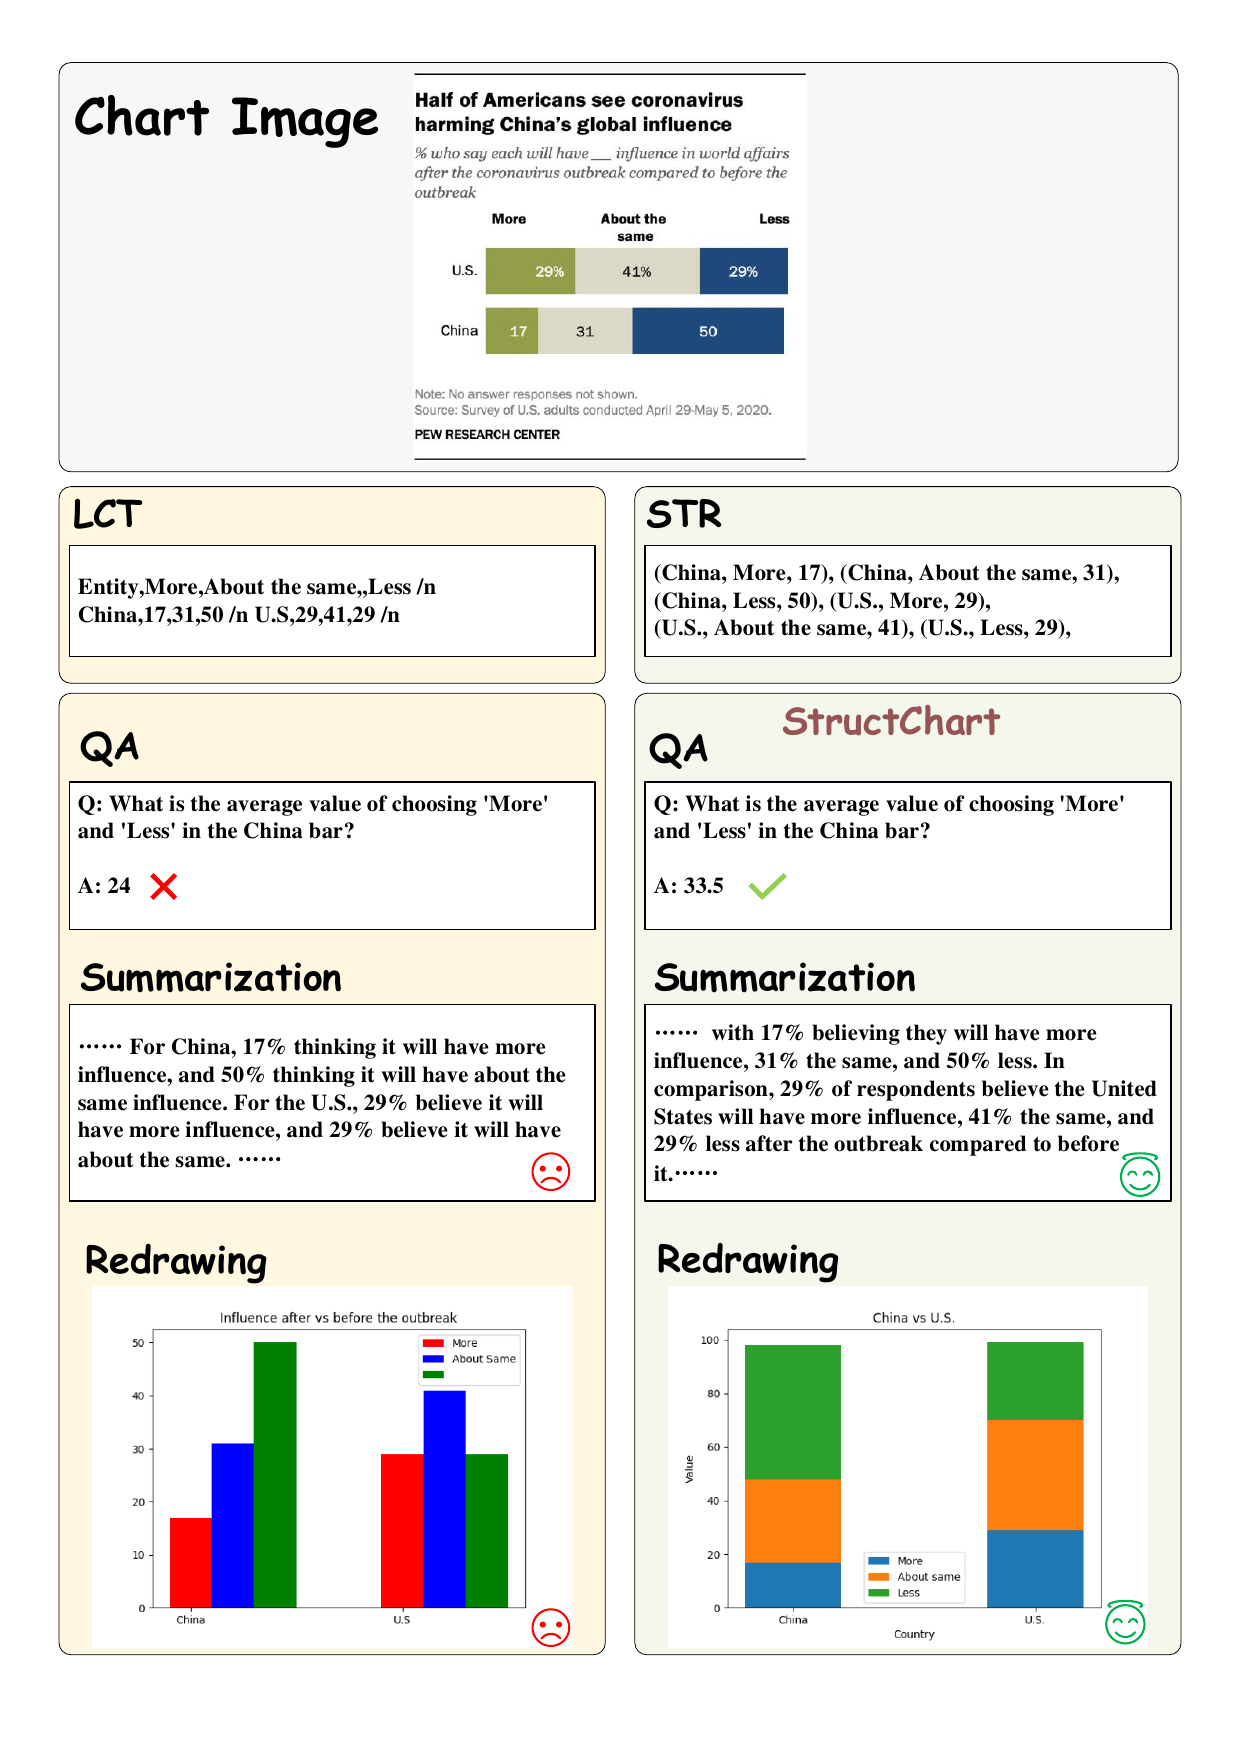}
\vspace{-5pt}
\caption{Visualization results (a comma introduced in LCT) using the proposed StructChart on downstream tasks with Linear CSV Tokens (LCT) v.s. Structured Triplet Representations (STR).}
\label{fig:lct_str_1}
\end{figure}

\begin{figure}[tb!]
\centering
\includegraphics[width=0.88\linewidth]{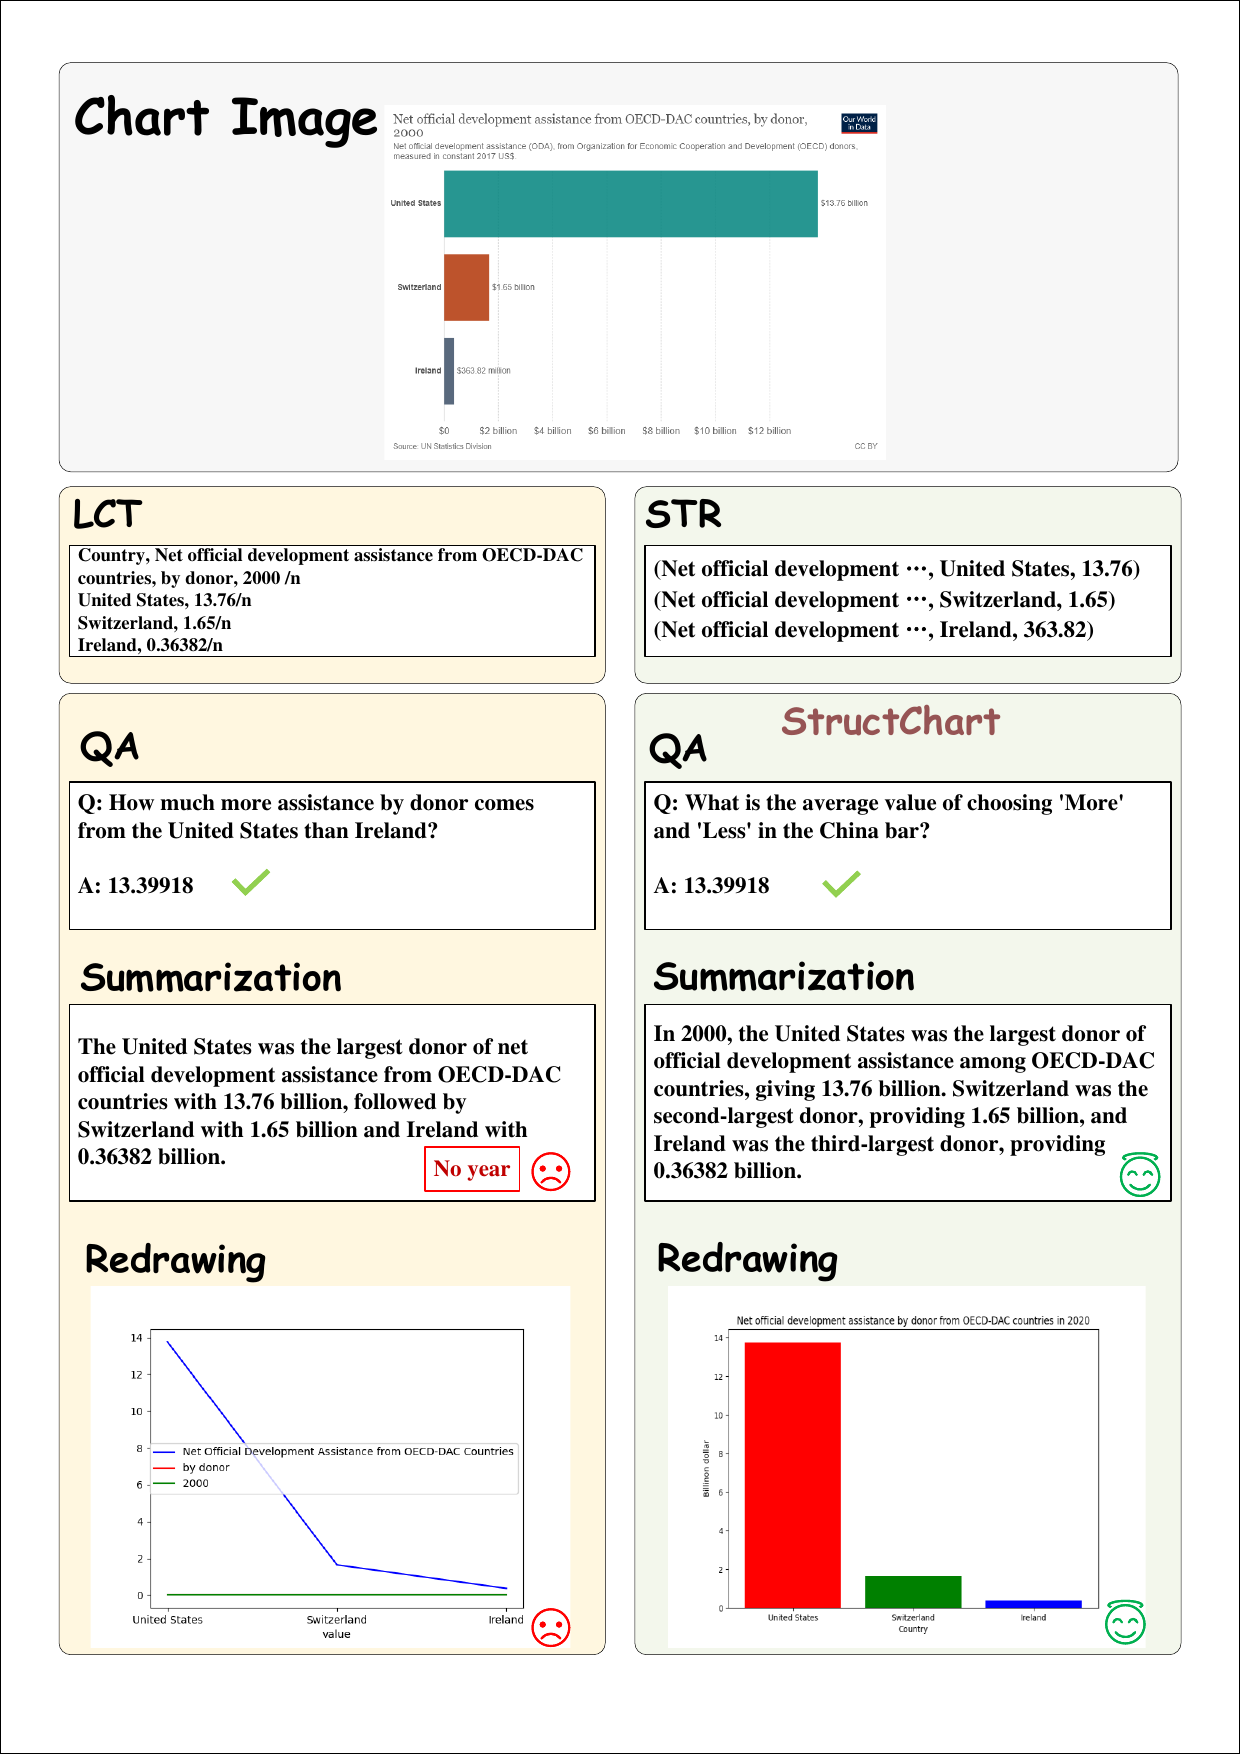}
\vspace{-5pt}
\caption{Visualization results (the separator comma itself is included in chart image) using the proposed StructChart on downstream tasks with Linear CSV Tokens (LCT) v.s. Structured Triplet Representations (STR).}
\label{fig:lct_str_2}
\end{figure}

\begin{figure}[tb!]
\centering
\includegraphics[width=0.88\linewidth]{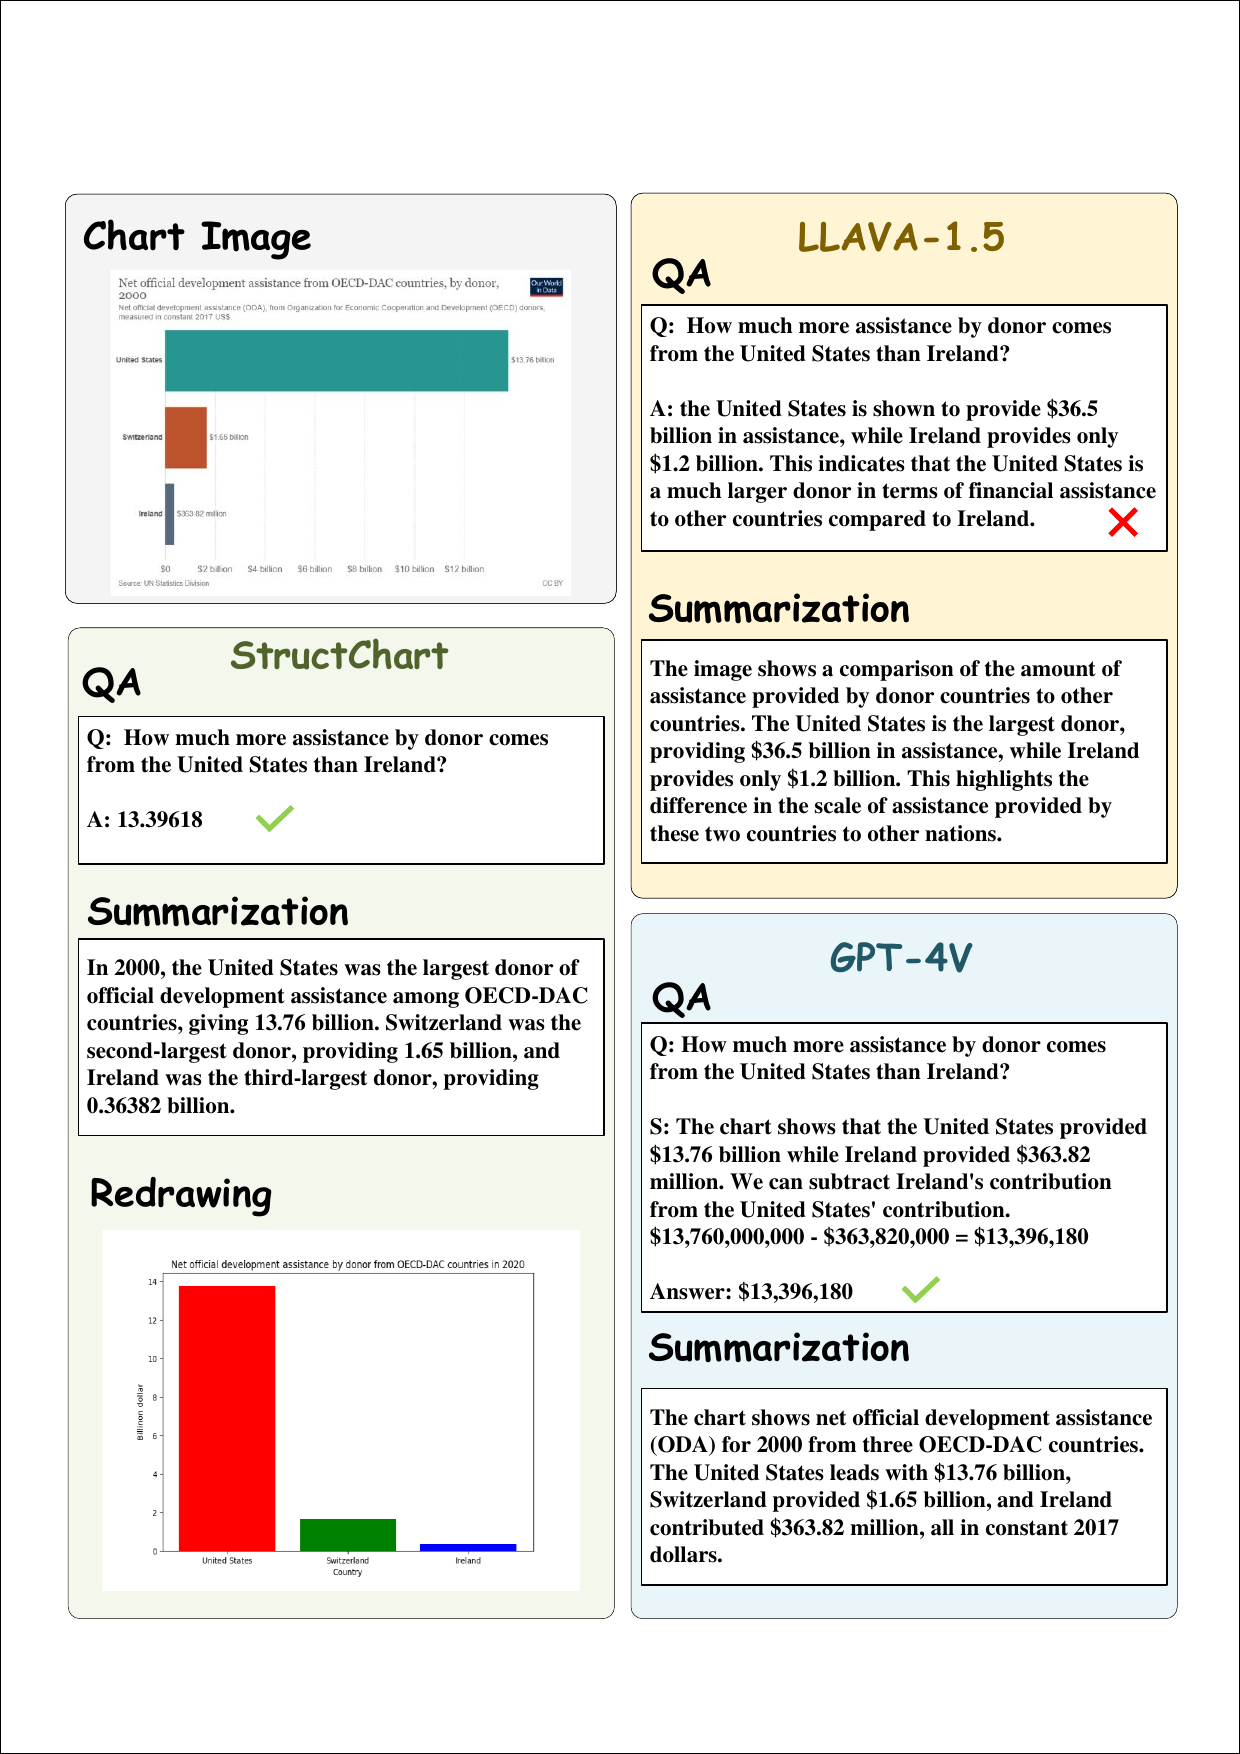}
\vspace{-5pt}
\caption{Visualization comparisons among StructChart, LLaVA-1.5~\citep{Liu2023VisualIT} and GPT-4V~\citep{OpenAI2023GPT4TR} on downstream tasks.}
\label{fig:gpt4v_1}
\end{figure}

\begin{figure}[tb!]
\centering
\includegraphics[width=0.88\linewidth]{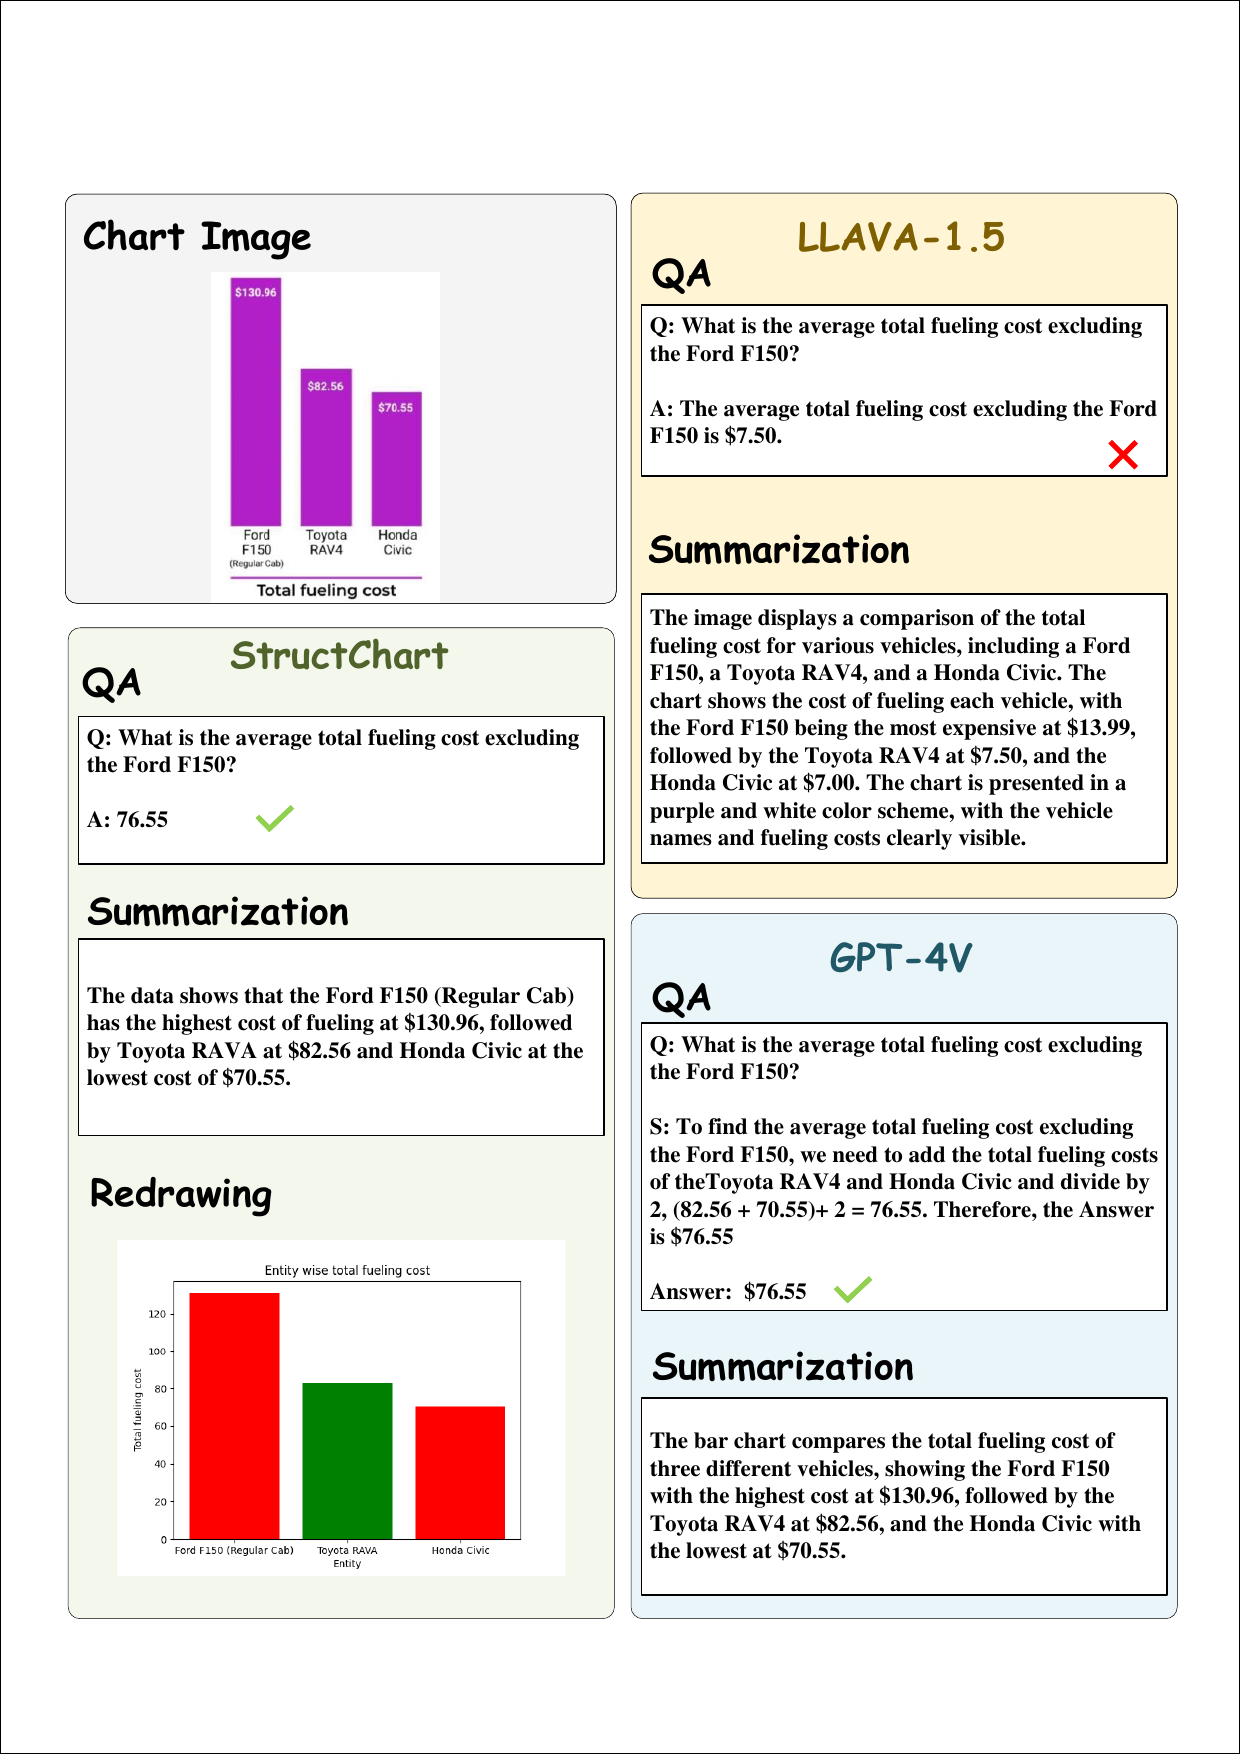}
\vspace{-5pt}
\caption{Visualization comparisons among StructChart, LLaVA-1.5~\citep{Liu2023VisualIT} and GPT-4V~\citep{OpenAI2023GPT4TR} on downstream tasks.}
\label{fig:gpt4v_2}
\end{figure}

\begin{figure}[tb!]
\centering
\includegraphics[width=0.88\linewidth]{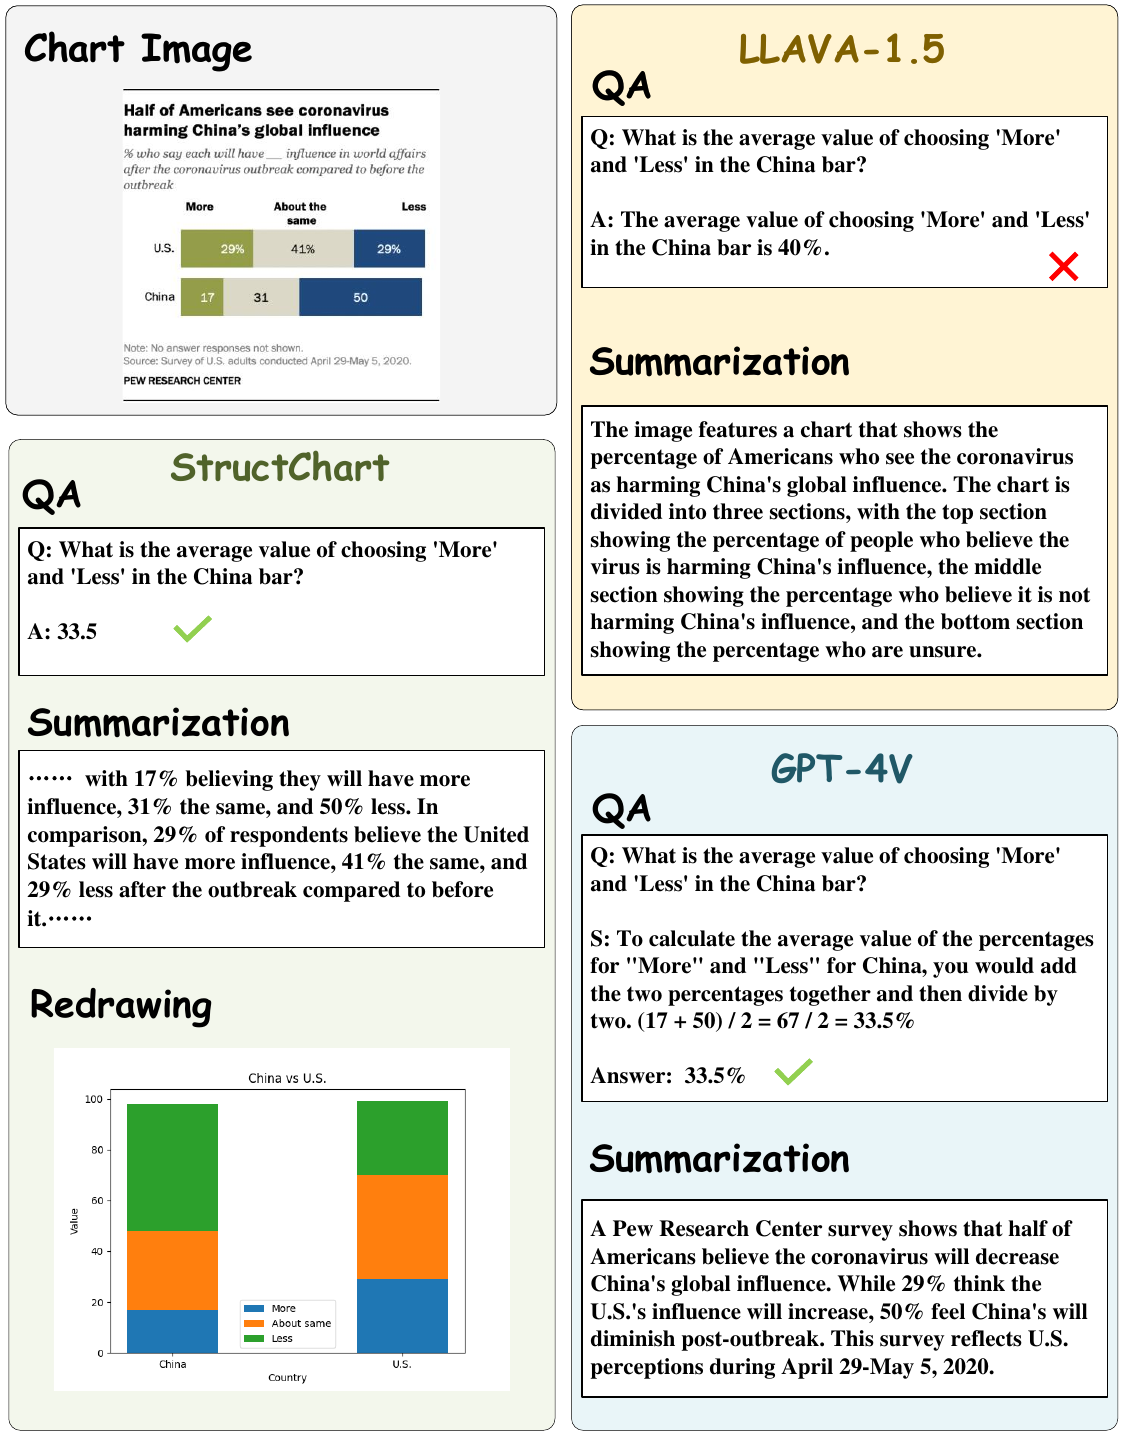}
\vspace{-5pt}
\caption{Visualization comparisons among StructChart, LLaVA-1.5~\citep{Liu2023VisualIT} and GPT-4V~\citep{OpenAI2023GPT4TR} on downstream tasks.}
\label{fig:gpt4v_3}
\end{figure}

\begin{figure}[tb!]
\centering
\includegraphics[width=0.81\linewidth]{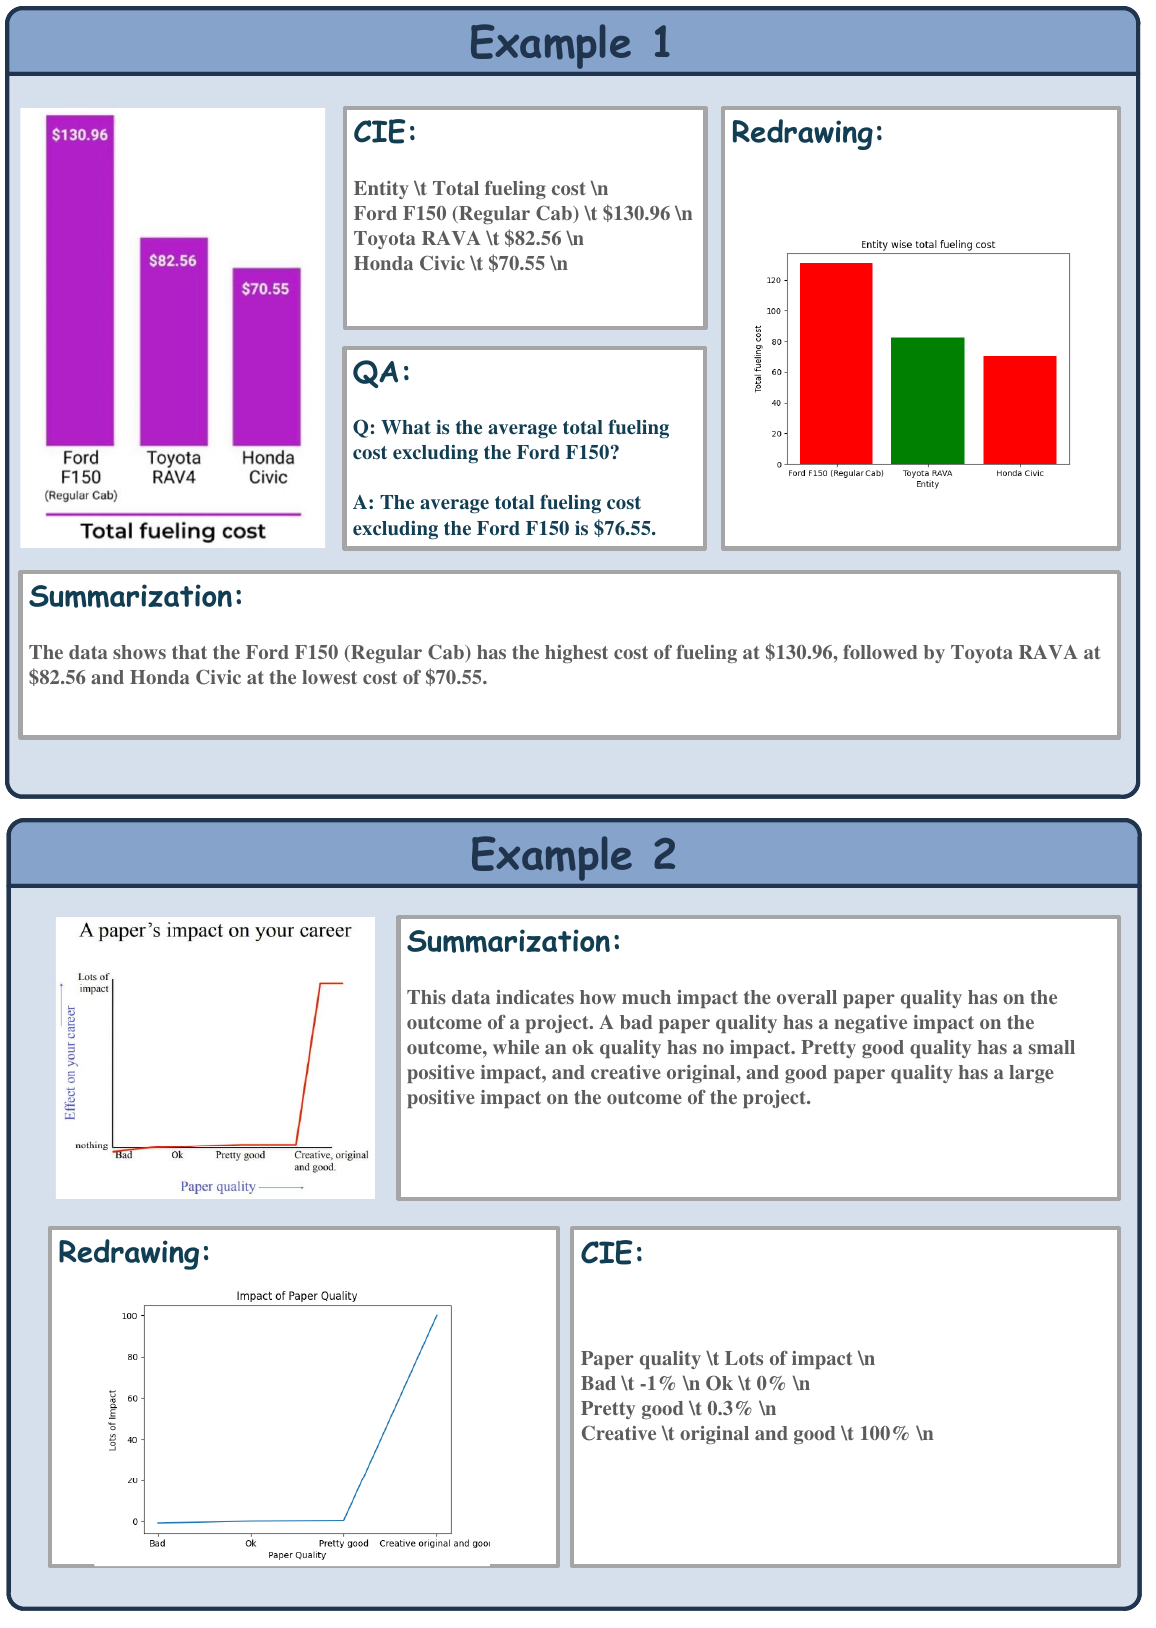}
\vspace{-5pt}
\caption{Visualization performance of StructChart on in-the-wild chart images.}
\label{fig:ood}
\end{figure}
}
